# Supplementary material for: Ultrastrong magnetic light-matter interaction with cavity mode engineering
Source: arXiv:2108.13266 ancillary file (2023-05-18)
Supplement: Supplementary file 1 [file SI.pdf]

# Supplementary Information: Ultrastrong magnetic light-matter interaction with cavity mode engineering

Hyeongrak Choi[1,*] and Dirk Englund[1,†]
[1]Research Laboratory of Electronics, Massachusetts Institute of Technology, Cambridge, Massachusetts 02139, USA
(Dated: May 18, 2023)

## SUPPLEMENTARY NOTE 1: ADDITIONAL MODE IN A DOUBLE RE-ENTRANT CAVITY

Our two explanations on double reentrant cavity modes consider two $\mathrm{TM}_{010}$ modes of reentrant cavities or the $\mathrm{TM}_{110}$ mode of a double reentrant cavity. In the latter point of view, when the reentrance gap $g$ is small, the resonance by two reentrances has a similar frequency with the $\mathrm{TM}_{110}$ mode of cylindrical cavity. The coupling between two modes produces symmetric and antisymmetric modes.

Figure S1 shows the resonance frequency of double reentrant cavities with $R = g = 100$ $\mu$m changing $h_r$. The blue and red circles describe the resonance frequencies of the simulated modes at each parameter. The mode with a frequency insensitive to $h_r$ originates from the $\mathrm{TM}_{110}$ mode of the cylindrical cavity. The other mode with a frequency that rapidly varies with $h_r$ is from the reentrance resonance. The larger $h_r$, the larger capacitance and inductance decrease $f$. We found the level anti-crossing at $h_r \approx 8.1$ mm, where the symmetric (anti-symmetric) mode has a higher (lower) frequency. The close-up inset fits the simulated data points with our two-mode coupling model. The fitted coupling frequency is 50 MHz.

In Fig. 6 of the main text, we included both modes for double reentrant cavities (yellow) and tapered double reentrant cavities (blue).

## SUPPLEMENTARY NOTE 2: $V_B$-SCALING OF RE-ENTRANT CAVITIES

In the main text, we find that $V_B \propto (R\ln(a/R))^2$ ($V_B \propto B_s^{-2}$). We compare this analytical expression with numerically simulated values. Figure S2 plots $V_B$ of the re-entrant cavities ($h = 10$ cm, $h_r = 8$ cm, $a = 2$ cm) changing $R$. We confirm the excellent agreement between the simulation result (blue circles) and $V_B/\lambda^3 = (0.8\ \mathrm{m}^{-2})\cdot(R\ln(a/R))^2$ (red dashed line). Note that the scaling cannot be fit to $\propto R$ or $\propto R^2$ (black dotted lines).

## SUPPLEMENTARY NOTE 3: MODIFICATION OF CAVITY DESIGNS

The cavity designs presented can be adjusted for target application, ease of fabrication, and operational frequencies. Figure S3 describes a few examples of cavity modification. For example, when inverse tapering of reentrances is not plausible, one can use step-profile reentrances (Fig. S3(a) and (b)). Step-profile reentrances produce more uniform field strength in $z$ near the narrow part compared to linearly tapered ones. For applications demanding a uniformly enhanced magnetic field, e.g., ensemble spin coupling, we can flatten the inner side of the reentrances (Fig. S3(c)). On the other hand, shortening double reentrances with an additional top reentrance helps to reduce the loss, but with additional complexity (Fig. S3(d)). Lastly, Fig. S3(e) presents a reentrant cavity with the field expulsion engineering.

## SUPPLEMENTARY NOTE 4: A HYBRID CAVITY DESIGN

Some applications benefit from dielectric cavities where the high-permittivity dielectric reduces the mode volume [S1]. Often, these cavities are shielded with a metallic enclosure to reduce radiation loss for high-$Q$ operation

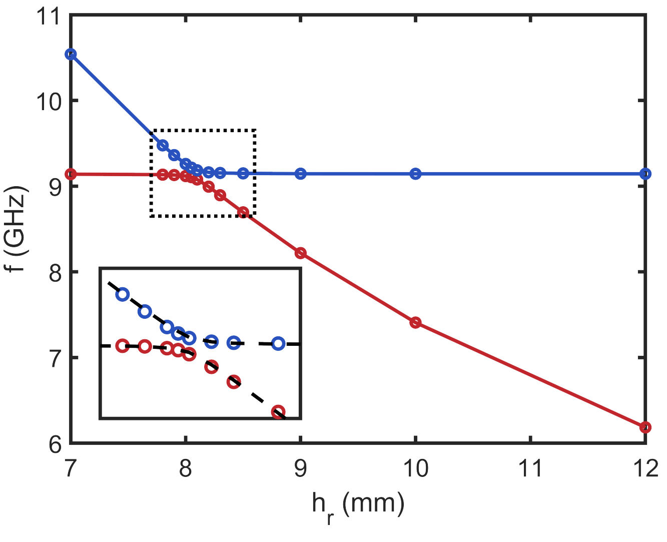


FIG. S1. **The two modes of double re-entrant cavities.** Blue (red) circles are the simulated values of resonant frequencies of high (low) frequency modes. (Inset) the black dashed line fits the data points near level anticrossing. $f = \frac{f_1+f_2\pm\Delta}{2} \pm \epsilon$, $f_1 = 9.14$ GHz, $f_2 = (9.14\ \mathrm{GHz}) + (1.12\ \mathrm{GHz}\cdot\mathrm{mm}^{-1})\cdot\left[(8.1\ \mathrm{mm}) - h_r\right]$, $\Delta = |f_1 - f_2|$, $\epsilon = \epsilon_0^2/\sqrt{\Delta^2+\epsilon_0^2}$, $\epsilon_0 = 0.05$ GHz.

[S2].

Our mode engineering techniques can also be applied to dielectric cavities. We present an exemplary design in Fig. S4(a). Two dielectric tubes (green) sandwich two thin metallic sheets that have a small gap between each other. Because the magnetic field of the $TE_{01\delta}$ mode should pass through the center, the sheets confine the field at the gap with high intensity.

Figures S4(b) and (c) show the in- and out-of-plane field distributions. We started from the dielectric cavity design of [S1], which originally had $V_B = 1.06 \times 10^{-3}$ ($\lambda^3$), and the hybrid design with field expulsion gives $V_B = 3.17 \times 10^{-4}$ ($\lambda^3$).

## SUPPLEMENTARY NOTE 5: A PRELIMINARY EXPERIMENTAL DEMONSTRATION

To verify the mode engineering method and the validity of the analysis, we fabricated and measured a copper cavity. With this preliminary demonstration, we confirm that the simulation and experiment agree in three key parameters: 1) resonance frequency ($f$), 2) quality factor ($Q$), and 3) the mode volume ($V_B$).

For the calculation of $V_B$, we used nitrogen vacancy (NV) centers in diamond to probe the microwave magnetic field of the cavity. The ground state of the NV centers is spin-triplet with 2.87 GHz zero field splitting [S3]. A strong microwave field at 2.87 GHz can coherently drive the spin state inducing Rabi oscillation. This oscillation can be observed with optically detected magnetic resonance (ODMR). We derive a microwave magnetic field from the Rabi oscillation frequency divided by the gyromagnetic ratio ($\sqrt{2}\cdot 28.02$ GHz/T, where $\sqrt{2}$ comes from the spin-1 Pauli matrix).

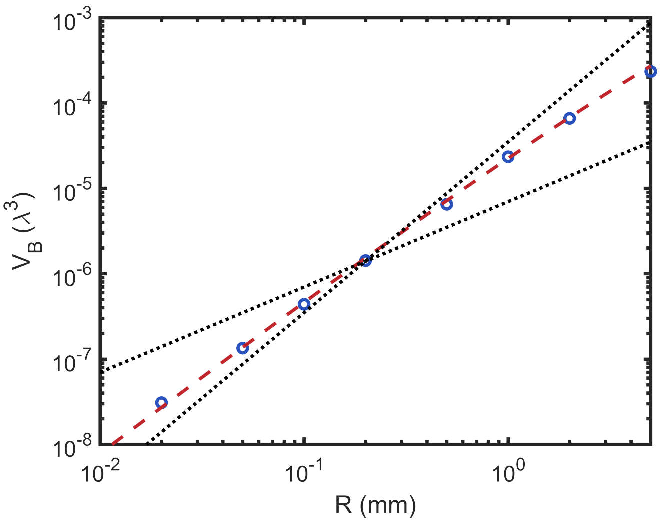


FIG. S2. **Scaling of $V_B$ on $R$ of re-entrant cavities.** Blue circles: simulated $V_B$s, red dashed line: $V_B/\lambda^3 = (0.8\ \mathrm{m}^{-2}) \cdot (R \ln(a/R))^2$, black dotted lines: $V_B/\lambda^3 = (35\ \mathrm{m}^{-2}) \cdot R^2$ and $V_B/\lambda^3 = (0.007\ \mathrm{m}^{-1}) \cdot R$.

Figure S5**a** shows the disassembled reentrant cavity. We designed the cavity based on Fig. 3(d) with the modification of height ($h = 1.9$ cm) to be resonant with NV centers ($f = 2.87$ GHz). We placed a $3 \times 3 \times 0.5$ mm$^3$ diamond between two reentrances. We soldered an open-ended SMA connector to the top plate (left) for probing the cavity field, and a hole at the bottom part (right) is for optically exciting and reading out NVs (see the inset). Figure S5**b** and S5**c** (close-up) plot the cavity magnetic field profile. As one can see, the magnetic field rapidly decays in the optical window, and the leakage through it is negligible as long as the bottom is thick enough (for our case, 5 mm).

We first characterized the cavity with a vector network analyzer (VNA, LibreVNA SEESII). Figure S6**a** plots the reflection ($S_{11}$) of the cavity. The reflection spectrum of a single-sided cavity is [S4],

$$S_{11} = e^{i[(f-f_0)\tau+b]} \cdot \frac{(1-\beta) + iQ_\mathrm{i}\Omega}{(1+\beta) + iQ_\mathrm{i}\Omega}, \quad \text{(S1)}$$

where $f_0$ is the resonance frequency, $\tau$ is the delay, $Q_i$ is the intrinsic quality factor, $\beta = \frac{Q_i}{Q} - 1$, $Q = \frac{Q_i \cdot Q_e}{Q_i + Q_e}$ is the loaded quality factor, $Q_e$ is the (extrinsic) coupling quality factor, and $\Omega = \frac{f}{f_0} - \frac{f_0}{f}$. We fit Eq. (S1) (line) to the measured spectrum (marker) in excellent agreement. The fit parameters are $f_0 = 2.8709$ GHz, $Q_\mathrm{i} = 2,421$, $\beta = 0.2322$, $b = -0.3220$, and $\tau = -2.457 \times 10^{-8}$. The measured $f_0$ and $Q_i$ are similar to the simulated value of 2.864 GHz and 3,169, respectively (the simulated $Q_i$ is based on the surface resistance room temperature Cu, $R_s = 15.1$ m$\Omega$).

Figure S6**b** shows the continuous-wave optically detected magnetic resonance (CW-ODMR). In this measurement, we drove the spin states of NVs ($|m_s = 0\rangle \leftrightarrow |m_s \neq 0\rangle$) with the cavity magnetic field and measured the fluorescence under 532 nm illumination. Because the $|m_s \neq 0\rangle$ state is darker due to the intersystem crossing (ISC) to the singlet state, the fluorescence drops when the microwave is resonant with the spins. We found four dips in the signal corresponding to four different orientations of NVs in the crystal split by the residual magnetic field in the system.

Setting the microwave at 2.871 GHz, we strongly drove

TABLE S1. Comparison of the simulation with experimentally measured values.

| | simulation | experiment |
|---|---|---|
| resonance frequency (GHz) | 2.864 | 2.871 |
| intrinsic quality factor | 3,169 | 2,421 |
| mode volume ($\lambda^3$) | $1.95 \times 10^{-3}$ | $1.75 \times 10^{-3}$ |
| (Rabi frequency (MHz) | 2.725 | 2.929) |

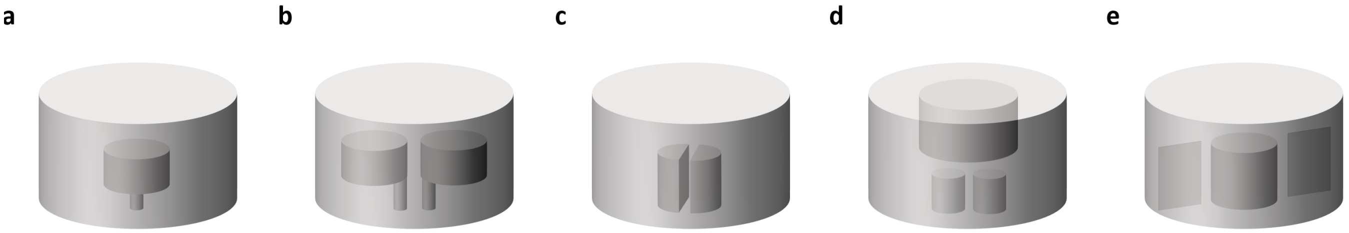


FIG. S3. **Modified cavity designs.** **a** Step-profile reentrant cavity. **b** Step-profile double reentrant cavity. **c** Flattened double reentrant cavity. **d**, **e** Cavity designs combining multiple features.

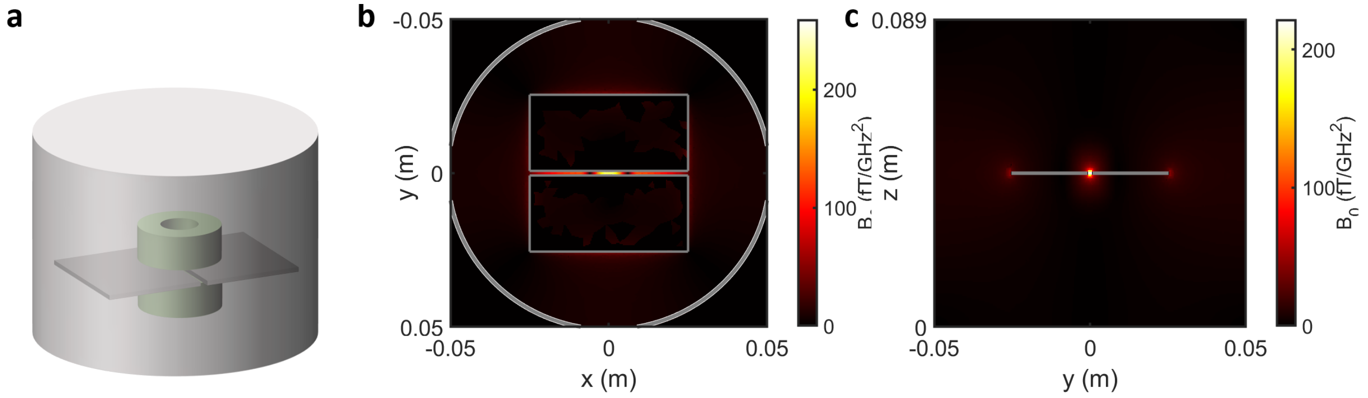


FIG. S4. **A hybrid cavity design.** **a** Two metallic plates with a small gap are between two dielectric cylinders. **b**, **c** Magnetic field of the $TE_{01\delta}$-like mode has a high strength at the gap.

(25 dBm) spins and measured the fluorescence. Fluorescence oscillates with driving time, as shown in Fig. S6**c** (Rabi oscillation). We fit the signal to the sum of three damped oscillations corresponding to the three groups of NVs that orient differently. The lowest oscillation frequency was 2.929 MHz, which is also in agreement with the simulated value of 2.725 MHz. In this calculation, we also included a factor of $\sqrt{2/3}$ derived from the relative orientation of the magnetic field and the spin (only the transverse component of the microwave drives the spin).

TABLE S1 summarizes the comparison of the experimentally measured parameters with the simulation. The mode volume of the cavity is with $\vec{r}_e$ at the center of the diamond. Experimentally measured $V_B = 1.75 \times 10^{-3}\lambda^3$ is close to simulated $1.95 \times 10^{-3}\lambda^3$.

## SUPPLEMENTARY NOTE 6: SIMULATION WITH A DIELECTRIC SUBSTRATE

Figure S7 describes the simulated cavity with a dielectric substrate. We added HEMEX sapphire post (1.75 cm × 2 mm × 100 $\mu$m) to the cavity of Fig. 5**b**. The magnetic field is measured at 5 $\mu$m away from the edge of the foil as Fig. 5**b**, considering the fabrication of a device.

## SUPPLEMENTARY REFERENCES

* choihr@mit.edu
† englund@mit.edu

[S1] E. R. Eisenach, J. F. Barry, M. F. O'Keeffe, J. M. Schloss, M. H. Steinecker, D. R. Englund, and D. A. Braje, Nature communications **12**, 1 (2021).

[S2] J. Krupka, K. Derzakowski, B. Riddle, and J. Baker-Jarvis, Measurement Science and Technology **9**, 1751 (1998).

[S3] M. W. Doherty, N. B. Manson, P. Delaney, F. Jelezko, J. Wrachtrup, and L. C. Hollenberg, Physics Reports **528**, 1 (2013).

[S4] R. S. Kwok and J.-F. Liang, IEEE Transactions on Microwave Theory and Techniques **47**, 111 (1999).

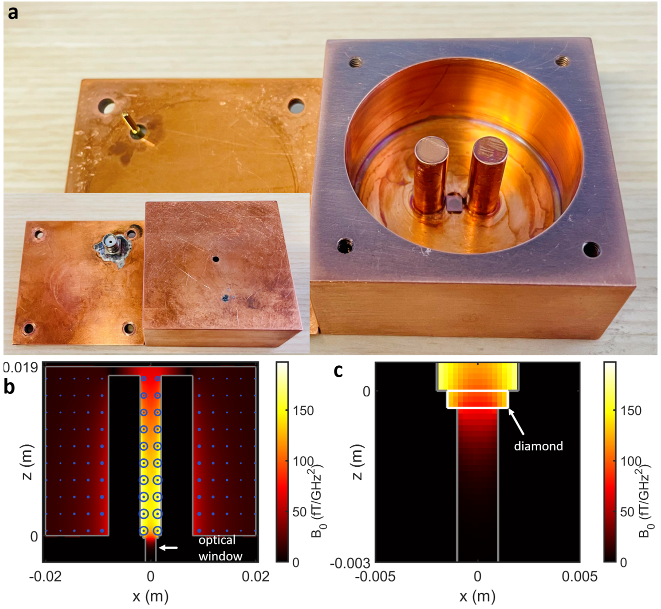


FIG. S5. **Experimental demonstration of a double reentrant cavity design.** **a** Top (left) and bottom (right) parts of fabricated copper cavity. The design is the same as Fig. 3(d) except $h = 1.9$ cm resulting in $f = 2.87$ GHz. The holes on the top and bottom are for in/out coupling and optical pumping, respectively. The inset shows the other side of the cavity components. We used an open-ended SMA to probe the cavity field. We locate a $3\times3\times0.5$ mm$^3$ diamond between two reentrances for measuring a cavity magnetic field. **b** Simulated magnetic field of the cavity. The magnetic field of the cavity mode quickly decays through the optical window, and the radiation loss from the window is negligible. **c** Close-up field distribution around the optical window and the diamond.

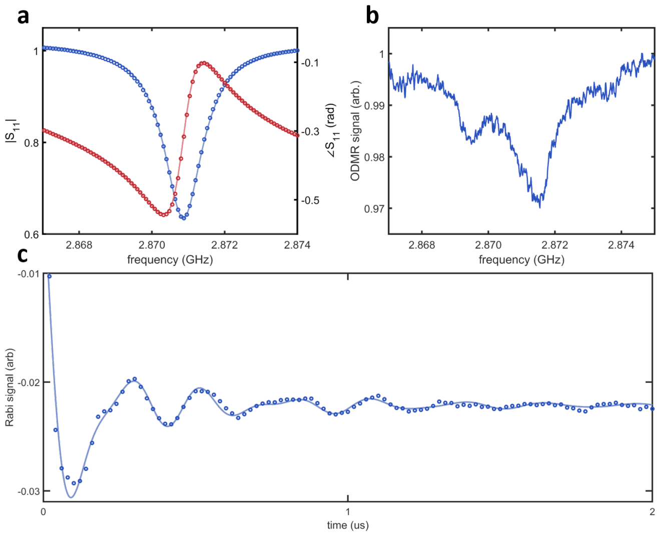


FIG. S6. **Cavity characterization with NV centers in diamond.** **a** Microwave cavity reflection spectrum, $S_{11}$ (marker: measured, line: fit). We used Eq. (S1) for the fitting. **b** Cavity-driven CW-ODMR signal. **c** Cavity-driven Rabi oscillation of NV centers. The markers are the measured data, and the line fits with $\Sigma_i A_i \cdot \exp(-t/\tau_i) \cdot \cos(\omega_i t + \phi_i) - 0.2214$

($A_{1,2,3} = 0.0243$, 0.001886, 0.002767, $\tau_{1,2,3} = 0.1002$, 0.7675, 0.4000, $\omega_{1,2,3} = 2\pi(2.929$, 3.519, 5.440), $\phi_{1,2,3} = 0.609$, 1.058, 1.422).

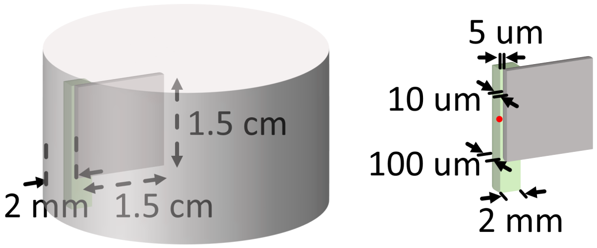


FIG. S7. **Simulated field-expulsion cavity with dielectric substrate.** (Left) field-expulsion cavity of Fig. 5**b** with HEMEX sapphire substrate ($\epsilon = 9.39$). (Right) detailed dimensions of the dielectric and the foil. The red circle shows the point where the magnetic field is measured for the calculation of $V_B$.
